# Supplementary material for: Enhanced Face Authentication With Separate Loss Functions
Source: arXiv:2302.11427 source file (2024-03-20)
Supplement: Supplementary file 1 [file appendix2.tex]

\chapter{Mã nguồn }
\label{Appendix2}

Đây là phụ lục 2.
