# Supplementary material for: Enhanced Face Authentication With Separate Loss Functions
Source: arXiv:2302.11427 source file (2024-03-20)
Supplement: Supplementary file 2 [file reassurances.tex]

\chapter*{Lời cam đoan}
\label{reassurances}

Tôi xin cam đoan đây là công trình nghiên cứu của riêng tôi. Các số liệu và kết quả nghiên cứu trong luận văn này là trung thực và không trùng lặp với các đề tài khác.
